# Supplementary material for: A Refreshed Similarity-based Upsampler for Direct High-Ratio Feature Upsampling
Source: arXiv:2407.02283 source file (2025-02-08)
Supplement: Supplementary file 1 [file supp.tex]

\clearpage
\setcounter{page}{1}
\maketitlesupplementary

\section{Implementation Details}

\subsection{Experimental Setup}
% \vspace{1mm}
% \noindent \textbf{Experimental Setup.} 

\noindent \textbf{Network Architectures.}  
We evaluate the upsampling methods on semantic/instance/panoptic segmentation tasks. For the semantic segmentation task, we conduct a comprehensive evaluation of various network architectures as follows: 

\noindent (a) PSPNet \cite{zhao2017pyramid} with ResNet50 \cite{he2016deep} as the backbone. The initial feature obtained by applying a ConvBlock to the image is used to guide the $\times 4$ upsampling of the final deep feature, as shown in \cref{fig:head} (a);

\noindent (b) Segmenter-S \cite{strudel2021segmenter} with the FCN-head \cite{long2015fully}. To guide the final $\times 4$ upsampling, we add an auxiliary ConvBlock on the image to generate the shallow guidance feature of channel size 64, as shown in \cref{fig:head} (b). The ConvBlock consists of two 3x3 Convolutions with a ReLU activation and a GroupNorm layer \cite{wu2018group} in between.

\noindent (c) SegFormer-B1 \cite{xie2021segformer}. For all comparing methods we adopt the iterative $\times 2$ upsampling as in \cref{fig:first} (a) while for ReSiFU we adopt the straightforward manner as in \cref{fig:head} (c);

\noindent (d) SegNext-B \cite{guo2022segnext}. SegNext produces 4 levels of features and upsamples C3 and C4 to concatenate with C2 for the final segmentation. Following the setting of SegFormer, We adopt iterative $\times 2$ upsamplings for all comparing methods, while using straightforward ones with C1 as the guidance feature, as shown in \cref{fig:head} (d).

\noindent (e) UNet-S5-D16 \cite{ronneberger2015u} with the FCN-head. We use the shallow feature C1 to guide the three $\times 2$ upsamplings in the decoding procedure, as shown in \cref{fig:head} (e).

% We use Mask RCNN \cite{he2017mask} and Panoptic FPN \cite{kirillov2019panoptic} for instance segmentation and panoptic segmentation, respectively. We modify the upsampling stages in their FPN necks \cite{lin2017feature}.

% For instance segmentation, we use Mask RCNN \cite{he2017mask} with ResNet50 as the backbone. We modify the upsampling stages in the FPN neck \cite{lin2017feature} and the ROI extractor. 

% For panoptic segmentation, we use Panoptic FPN \cite{kirillov2019panoptic} with ResNet50 as the backbone. We also modify the upsampling stages in the FPN neck.

We employ Mask RCNN \cite{he2017mask} with ResNet50 as the network architecture for instance segmentation. In this approach, we modify the upsampling stages within the FPN neck \cite{lin2017feature} as well as the ROI extractor. There are three $\times 2$ upsampling modules in the FPN and a $\times 2$ one in the ROI extractor. Regarding panoptic segmentation, we utilize Panoptic FPN \cite{kirillov2019panoptic} with ResNet50 as the backbone. Similar to instance segmentation, we also make adjustments to the three upsampling stages within the FPN neck. 

\vspace{1mm}
\noindent \textbf{Training Protocols.} For semantic segmentation, we adopt the Cityscapes \cite{cordts2016cityscapes} dataset for UNet and adopt the ADE20K \cite{zhou2017scene} dataset for the other network architectures. The MS COCO \cite{lin2014microsoft} dataset is used for instance and panoptic segmentation tasks. The training protocols are based on MMSegmentation \cite{mmseg2020} and MMDetection \cite{mmdetection}, ensuring the reproducibility of all experiments. 

 \vspace{1mm}
\noindent \textbf{Evaluation Metrics.}
For semantic segmentation, we report the mean IoU (mIoU), mean pixel accuracy (mAcc), and boundary IoU (bIoU) \cite{cheng2021boundary} metrics. We calculate bIoU following the codes in \cite{lai2023denoising} and set the pixel distance parameter to $2\%$ as in \cite{cheng2021boundary}. For instance segmentation, we report mask average precision (AP) as well as AP$_{50}$, AP$_{75}$ (averaged over IoU thresholds), AP$_{S}$, AP$_{M}$, and AP$_{L}$ (at different scales). For panoptic segmentation, we report panoptic quality (PQ), PQ on things (PQ$^{th}$), PQ on stuff (PQ$^{st}$), segmentation quality (SQ), and recognition quality (RQ) \cite{kirillov2019panoptic}.  %, thus the results would show slight differences as reported in \cite{liu2023learning}.

\vspace{1mm}
\noindent \textbf{Implementation Details.}
We set the radius $r$ in GF to 8, and $\epsilon$ to 0.001. For the design of ConvBlock in PCD-ConvBlock, we use a ``ReLU-Conv1x1" block for the semantic segmentation task, while we use a ``ReLU-Conv1x1-ReLU-GroupNorm-Conv1x1'' block for the instance and panoptic segmentation tasks. In them, the intermediate channel size is set to 128. For the backbones with shallow guidance features, such as PSPNet and Segmenter, we set the projection dimension $d$ to 32. For other scenarios, we set $d$ to 128. \hippo{More details about experimental setups can be found in \textit{SM}.}

% \subsection{Main Results}
% \paragraph{Semantic Segmentation.}
% Semantic segmentation is a representative dense prediction task that assigns pixel-wise prediction to images. For various network architectures solving this task, feature upsampling plays a vital role in different manners. 
% \paragraph{Instance/Panoptic Segmentation}

% \subsection{Ablation Study} \label{sec:ablation}

% \input{misc/table_instance}
% \input{misc/fig_vis_ins_pano}
% \input{misc/tab_ablation}
