# Supplementary material for: A Refreshed Similarity-based Upsampler for Direct High-Ratio Feature Upsampling
Source: arXiv:2407.02283 source file (2025-02-08)
Supplement: Supplementary file 2 [file X_suppl.tex]

\clearpage
\setcounter{page}{1}
\maketitlesupplementary
